# Supplementary material for: High-speed synchrotron X-ray imaging of melt pool dynamics during ultrasonic melt processing of Al6061
Source: arXiv:2407.10282 source file (2024-07-14)
Supplement: Supplementary file 1 [file Supplementary_Material.pdf]

# High-speed synchrotron X-ray imaging of melt pool dynamics during ultrasonic melt processing of Al6061

Lovejoy Mutswatiwa[1], Lauren Katch[1], Nathan John Kizer[1],
Judith Anne Todd[1], Tao Sun[2], Samuel James Clark[3],
Kamel Fezzaa[3], Jordan Lum[4], David Matthew Stobbe[4],
Griffin Jones[5], Kenneth Charles Meinert Jr.[5],
Andrea Paola Argüelles[1], Christopher Micheal Kube[1]*

[1]Engineering Science and Mechanics, The Pennsylvania State University, 212 Earth and Engineering Sciences Building, University Park, 16802, PA, USA.
[2]Materials Science and Engineering, University of Virginia, Wilsdorf Hall, 395 McCormick Road, Charlottesville, 22904, Virginia, USA.
[3]X-ray Science Division, Advanced Photon Source, Argonne National Laboratory, Lemont, IL, 60439, USA.
[4]Lawrence Livermore National Laboratory, 7000 East Ave, Livermore, 94550, CA, USA.
[5]Applied Research Laboratory, The Pennsylvania State University, 230 Innovation Blvd, University Park, 16802, PA, USA.

*Corresponding author(s). E-mail(s): kube@psu.edu;

## SUPPLEMENTARY MATERIAL

**Other supplementary materials for this manuscript include the following:**

- **High-speed Synchrotron X-ray videos of laser-generated Al6061 melt pool with and without applied sonication.**
- **Flow 3D simulation videos of melt pool dynamics of a single spot laser weld with and without sonication.**

Experimental setup at sector 32-ID-B at the Advanced Photon Source (APS), Argonne National Laboratory.

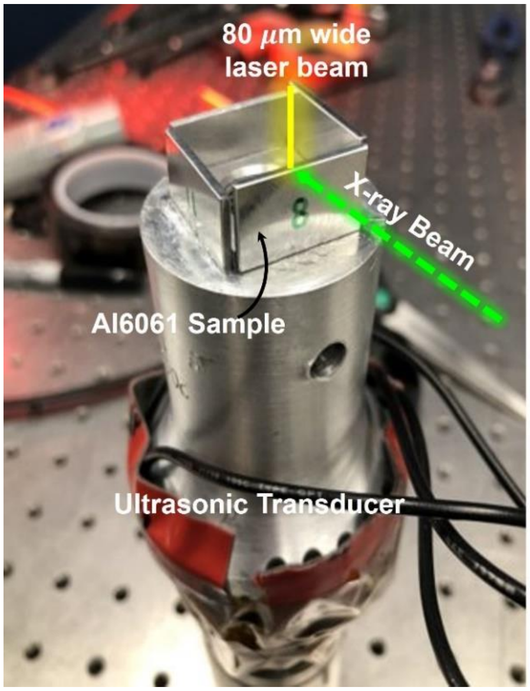


**Figure 1:** High-power ultrasonic transducer with four Al6061 samples adhered on top of the transducer horn. The Al6061 sample labeled 8 in the figure had a length of 20 mm, a height of 12 mm, and a thickness of 1.5 mm. The transducer was operated at its first-order longitudinal resonant frequency of 20.2 kHz.

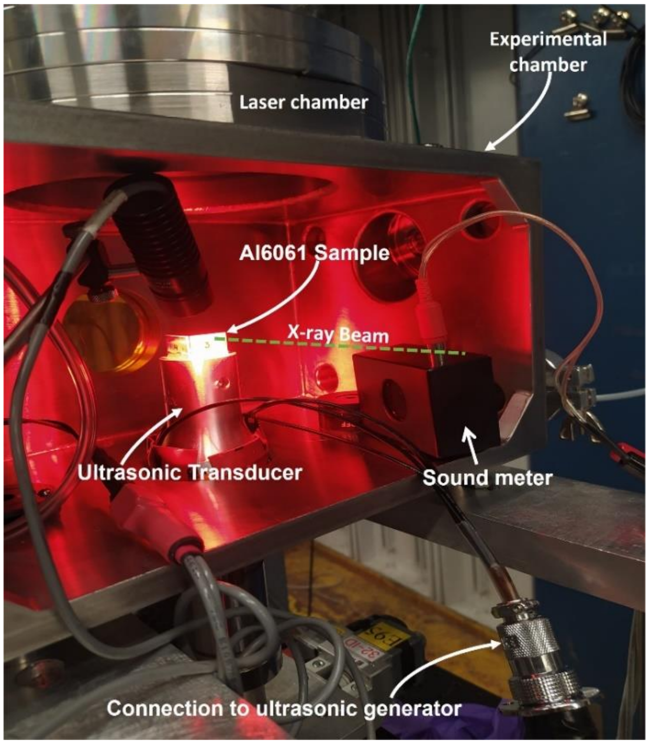


**Figure 2:** The experiment test chamber at Sector 32-ID-B at APS, showing the X-ray beam and Al6061 test specimen orientation.

## Flow3D Simulation

- Simulation time: 1.3 millisecond
- Laser on time: 0.8 milliseconds
- Laser power: 350 W
- Laser spot size: 80 microns
- Evaporation pressure coefficients: A = 31000 $g/(cm * s^2)$, B = 8
- Rising pressure magnification: 0.2
- Sonication amplitude: 8 µm
- Mesh size: 4 µm.
- Execution time ~ 15 hours
- Simulation domain (LxWxH): 0.5 x 0.5 x 0.8 mm
- Fluid characteristics: Laminar flow with temperature-dependent density.

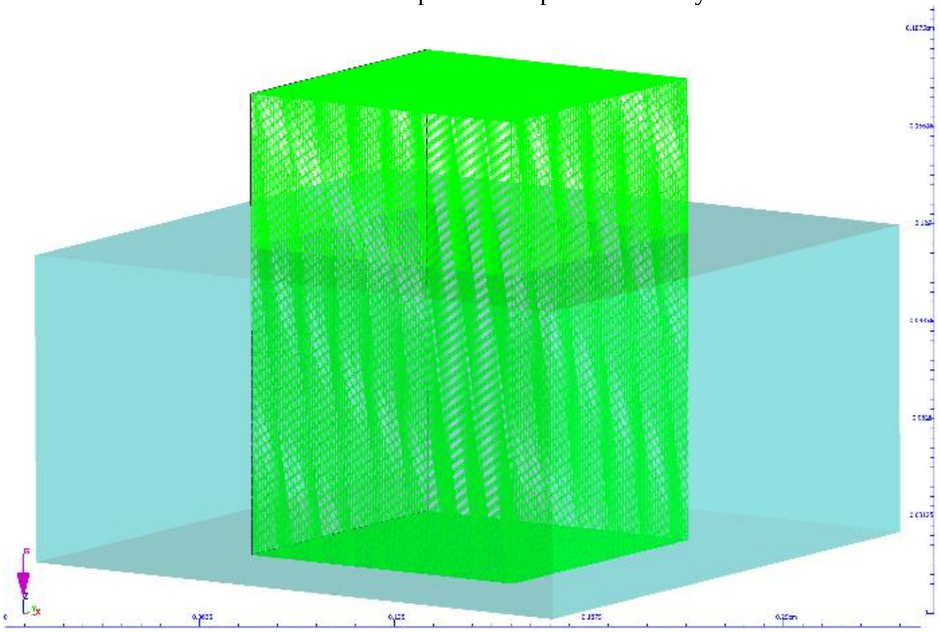

**Figure 3:** Flow 3D model for a single-spot laser weld simulation

**Bubble and phase change model.**

Figure 3 shows the orientation of the simulation model used in this study. The simulations used constant-pressure bubbles with a vaporization option in the bubble and phase change model under the physics widget. This model allows phase change due to evaporation and facilitates recoil pressure development, leading to keyhole melt pools. At pressures below the vapor pressure of molten Al6061, constant-pressure bubbles can be formed under this model. To accommodate phase change (i.e., evaporation and condensation, Flow 3D computes the vapor saturation pressure as a function of temperature based on the Clapeyron equation shown in Eq 1.

$$P^{sat} = PV1 * \exp\left[\frac{(\frac{1}{T} - \frac{1}{TV1})}{TVEXT}\right] \quad \textbf{Eq. 1}$$

Where PV1 and TV1 are points on the saturation curve, and TVEXT is a constant given by,

$$TVEXT = \frac{(\gamma - 1){C_V}^{vap}}{Latent\ heat\ of\ fusion} \quad \textbf{Eq. 2}$$

${C_V}^{vap}$ and $\gamma$ are the specific heat at constant volume and specific heat ratio, respectively. Figure 4 shows the dependence of vapor saturation pressure on temperature in molten aluminum, which was reported by Stull et al. [1]. Figure 4 was used to define the values of PV1 and TV1. The specific heat ratio of 2.1 was used in these aluminum simulations.

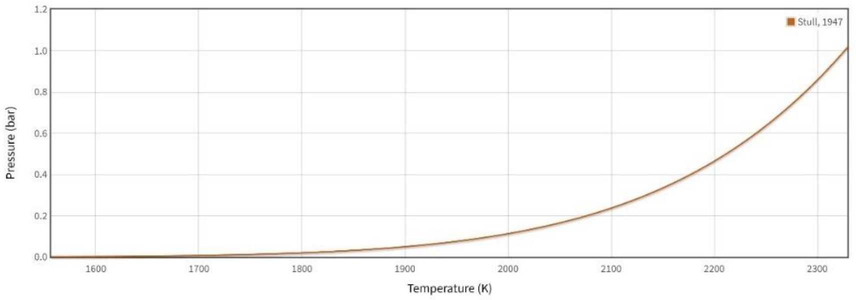


t

**Figure 4:** Molten aluminum vapor pressure-temperature dependence Stull et al. [1].

**Cavitation model**

These simulations used the active inertial cavitation model, which allows cavitation volume tracking and void opening. The cavitating void region may open in the fluid when the local pressure drops below the user-defined critical value, which is called the cavitation pressure. Though computationally expensive, the active inertial cavitation model more accurately predicts cavitation since the opening of the void relaxes the fluid pressure in the vicinity and may reduce further cavitation in the surrounding fluid. The formation rate of cavitation bubbles is controlled by an empirical parameter called characteristic time, introduced in the bubble and phase change section. The smaller the characteristic time, the higher the bubble formation and dissipation rate. The characteristic time defines the rate of bubble formation in the molten metal and is validated with experimental observations. Based on the cavitation bubble formation observed in high-speed synchrotron X-ray images of laser-generated melt pools, a characteristic time of 0.000125 seconds was defined for the formation of cavitation bubbles. A constant cavitation pressure of $1.03\ x\ 10\text{^}6\ dyne/cm^2$ was set in our simulations. Variable pressure bubbles (i.e., thermal bubbles) could be computed based on the Clausius-Clapeyron equation; however, the Flow 3D Additive Manufacturing software package does not allow thermal bubbles with phase change yet. The cavitation volume is computed using the following expression:

$$\frac{DV_{cav}}{Dt} = C_{av_{Production}} - C_{av_{dissipation}}$$

where,

$$C_{av_{Production}} = C_e \frac{E_{turb}}{\sigma} \rho_l \rho_v \sqrt{\left[\frac{2}{3}\frac{P_{cav} - P}{\rho_l}\right]} (1 - f_{cav})$$

and

$$C_{av_{dissipation}} = C_c \frac{E_{turb}}{\sigma} {\rho_l}^2 \sqrt{\left[\frac{2}{3}\frac{P - P_{cav}}{\rho_l}\right]} (f_{cav})$$

$V_{cav}$ is the computed cavitation volume fraction, $C_e$ and $C_c$ are the evaporation and condensation coefficients, respectively. $E_{turb}$ is the turbulent kinetic energy (or 10% of the total energy if no turbulent occurs), $\sigma$ is the surface tension coefficient, $P_{cav}$ is the user-defined cavitation pressure, P is the local fluid pressure, and $f_{cav}$ is the mass fraction of cavitation in the computational cell. $\rho_l$ and $\rho_v$ are the densities of the liquid and vapor, respectively.

**Gravity and non-inertial reference frame**

To simulate ultrasonic vibrations in Flow 3D AM, the non-inertial reference frame with harmonic oscillations was activated. A linear acceleration in the vertical direction (i.e., along the Z axis) was defined as;

$$a = -f^2 \times d \times \sin(f \times t - \emptyset) \qquad \textbf{Eq. 3}$$

where *f* is the angular frequency, *d* is the displacement amplitude, *t* is time, and $\emptyset$ is the phase. Similar to our experiments, an excitation frequency of 20.2 kHz corresponding to an angular frequency of $40400\pi\,\frac{\text{rad}}{\text{sec}}$, d a displacement amplitude of 8 $\mu m$ were used in the simulations. An initial gravity of $-981\ cm/s^2$ was defined along the Z direction.

**Surface tension model**

Bainbridge et al. [2] determined the surface tension of pure aluminum and aluminum alloys using the sessile drop method. Al6061 has Mg and Si as major alloying elements and Bainbridge et al.'s [2] findings show that its surface tension is in the 0.41 - 0.52 N/m range at the liquidus temperature (See Figure 6). Pure aluminum surface tension was measured to be 0.9 N/m, and adding alloying elements was observed to reduce the surface tension. In addition

to Mg and Si, Al6061 alloy has several other alloying elements such as Fe, Cu, Ti, Mn, Cr, Zn, etc.; therefore, its surface tension is expected to be lower than 0.52 N/m. Therefore, a surface tension of 0.45 N/m was used in our simulations. The surface tension is also temperature-dependent, according to

$$\sigma = \sigma_0 - \frac{d\sigma}{dT}(T - T^*) \quad \textbf{Eq. 4}$$

where, $\sigma$ is the computed surface tension, $\sigma_0$ is the surface tension at the liquidus temperature, T is the local temperature, $T^*$ is the user-defined reference temperature and $\frac{d\sigma}{dT}$ is the surface tension temperature dependence rate. The surface tension temperature dependence rate is defined as a coefficient in Flow 3D, and it was set at 0.001 g/s^2/K in our simulations.

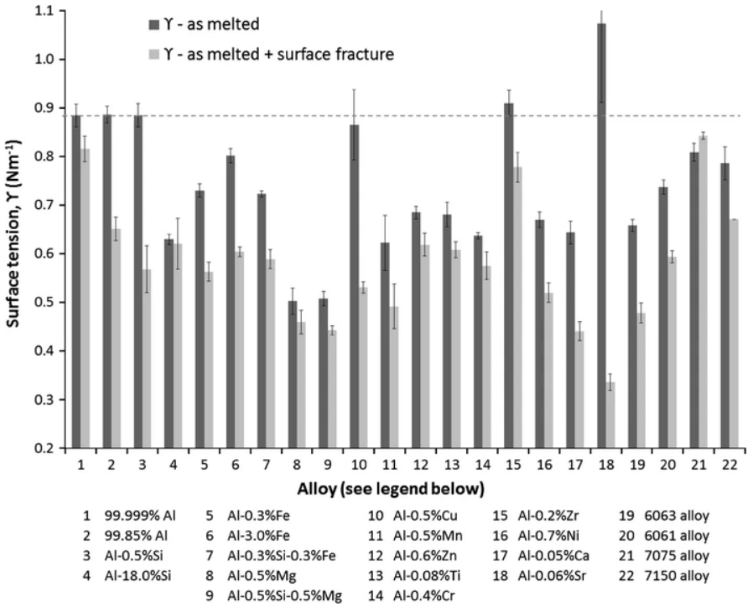


**Figure 5: Surface Tension of Molten Aluminum and Aluminum Alloys at Liquidus Temperatures Bainbridge et al. [2].**

**Underlying Assumptions**

The molten metal in the melt pool is considered a Newtonian fluid with laminar flow characteristics.

## Electron Backscattered Diffraction Analysis and Optical Imaging

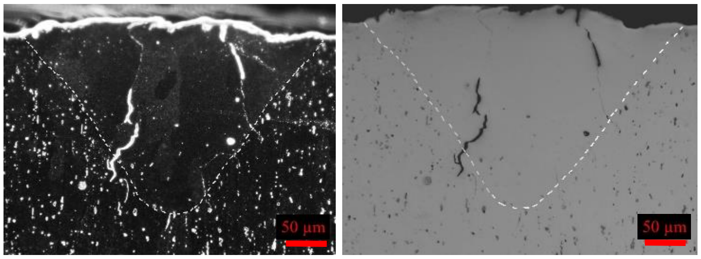


**a** **b**

**Figure 6:** Optical images of stationary laser-generated melt pool without sonication in **(a)** dark and **(b)** light fields. The final polishing of the Al6061 sample was conducted using the Final A polishing pad with 0.04 µm colloidal silica suspension for 12 hours.

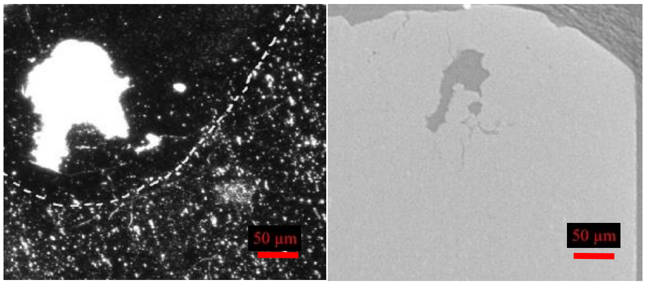


a b

**Figure 8:** **(a)** Optical image of stationary laser-generated melt pool with sonication in the dark field. **(b)** X-ray computed tomography frame of a melt pools generated on a vibrating substrate showing cavitation induced pores.

## REFERENCES

1. Stull, Daniel R., *Vapor Pressure of Pure Substances. Organic and Inorganic Compounds*, Ind. Eng. Chem., 1947, 39, 4, 517-540, https://doi.org/10.1021/ie50448a022.

2. Bainbridge, I.F., Taylor, J.A. The Surface Tension of Pure Aluminum and Aluminum Alloys. *Metall Mater Trans A* 44, 3901–3909 (2013). https://doi.org/10.1007/s11661-013-1696-9
